# Supplementary material for: Dipolar coupling of nanoparticle-molecule assemblies: An efficient approach for studying strong coupling
Source: arXiv:2101.05160 source file (2021-01-13)
Supplement: Supplementary file 1 [file supplementary-information.pdf]

# Supplementary Material

## Dipolar coupling of nanoparticle-molecule assemblies: An efficient approach for studying strong coupling

Jakub Fojt, Tuomas P. Rossi, Tomasz J. Antosiewicz, Mikael Kuisma, and Paul Erhart

## Contents

**Supplementary Figures** **2**
1. Parameters and their uncertainties extracted from Bayesian fits to the spectra of the coupled $Al_{201}$ NP-benzene system . . . 2
2. Spectra of the coupled $Al_{201}$ NP-benzene system, with varying NP-molecule distance, fitted to the coupled oscillator model . . . 3

**Supplementary Tables** **4**
1. Prior distributions of parameters in the Bayesian fitting scheme . . . 4

**Supplementary Notes** **5**
1. Fitting of spectra . . . 5

# Supplementary Figures

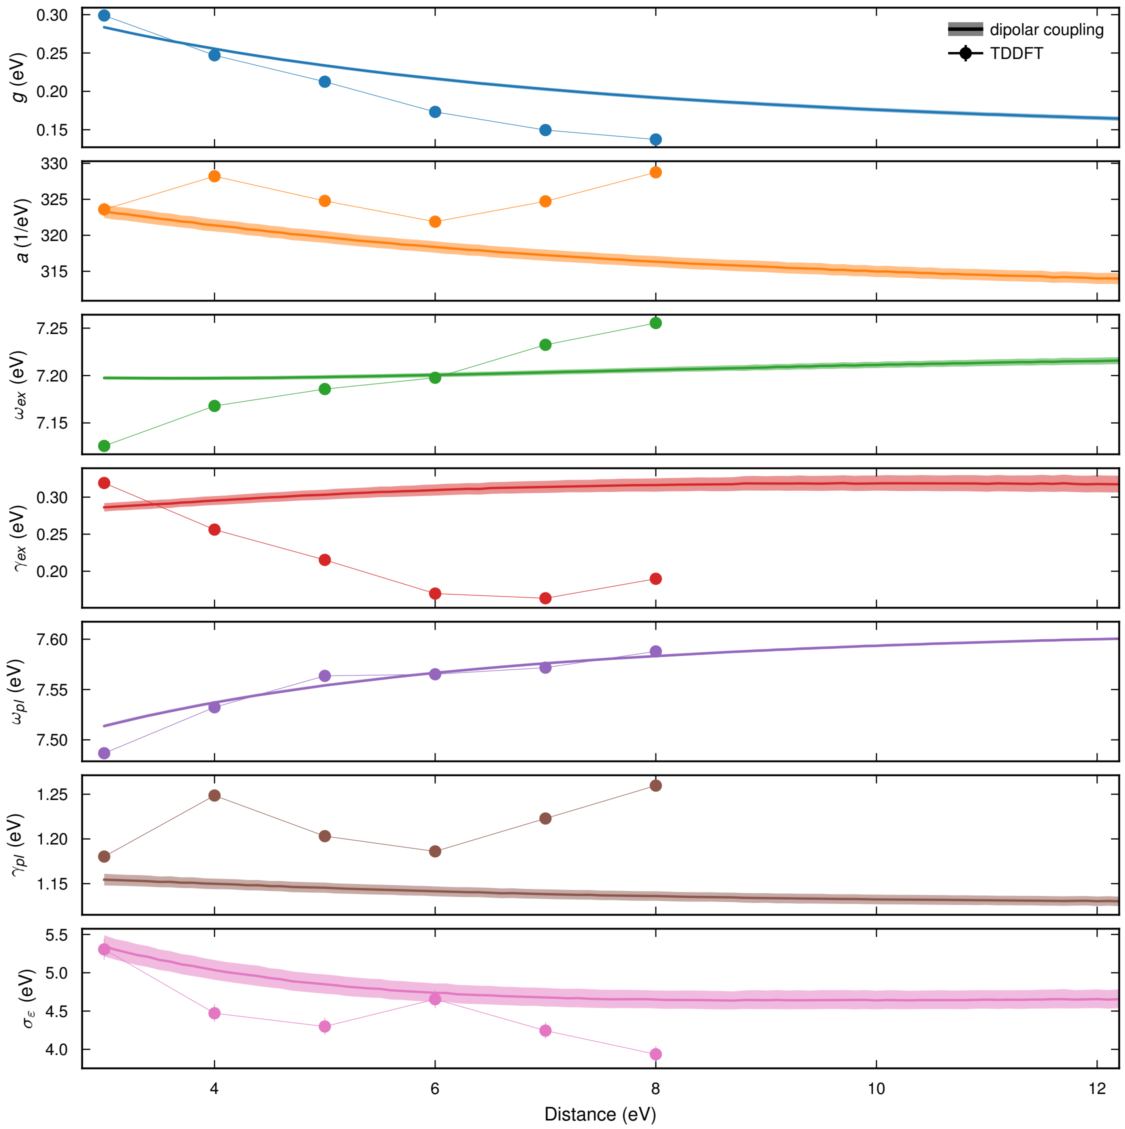


Supplementary Figure 1: **Parameters and their uncertainties extracted from Bayesian fits to the spectra of the coupled $Al_{201}$ NP-benzene system.** The model and fitting scheme are described in Supplementary Note 1. The general trend is that the fits vary smoothly with distance for the DC data, while there is significant scatter for TDDFT. The scatter and the different trends in $\omega_{\rm ex}$ and $\gamma_{\rm ex}$ in TDDFT data originate partially from the numerical inaccuracy of the spectrum due the localized basis sets changing with varying distance.

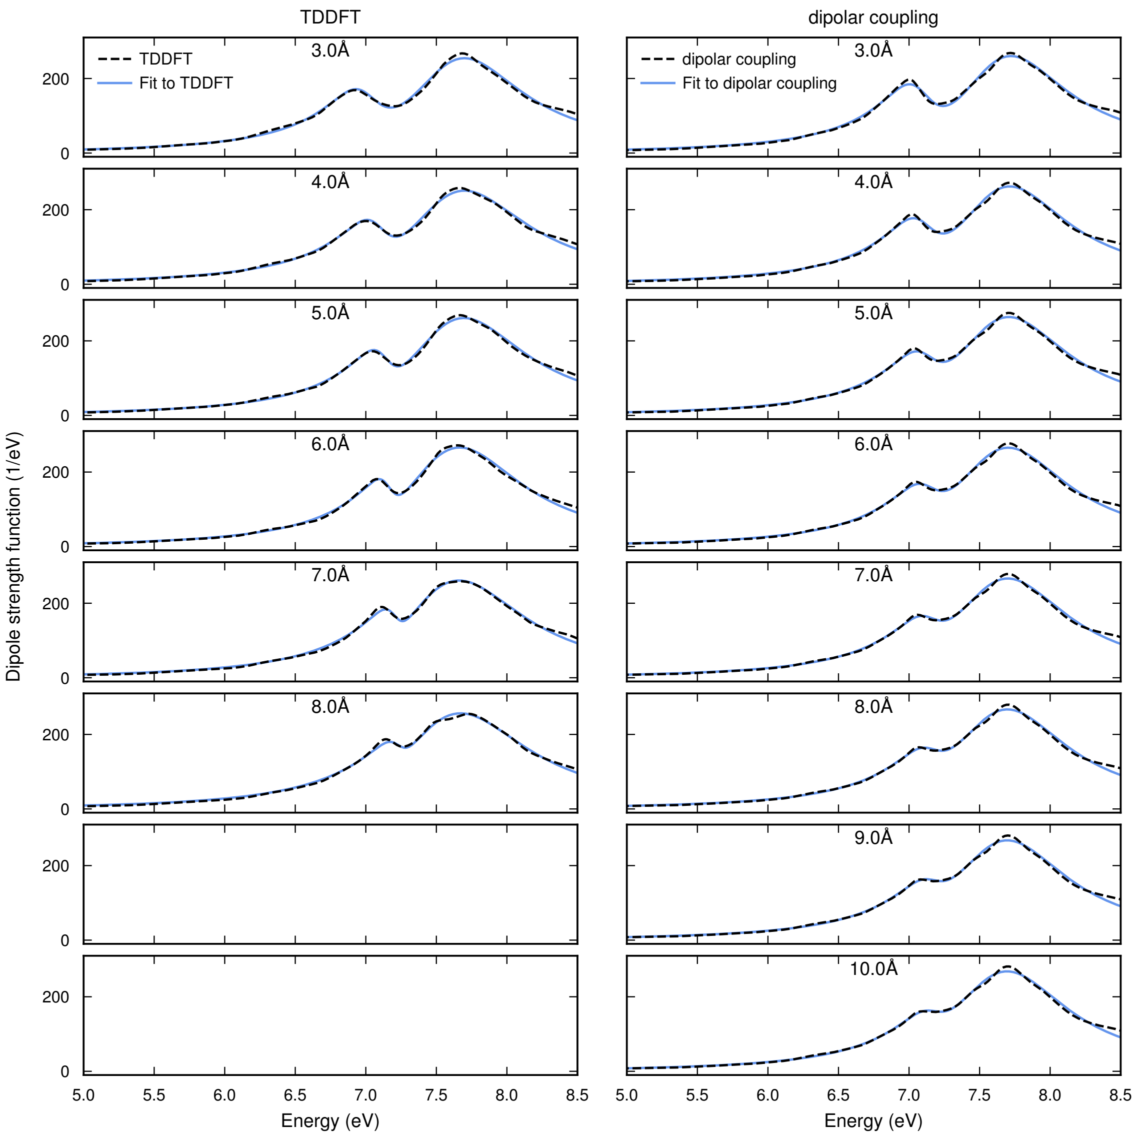


Supplementary Figure 2: **Spectra of the coupled $Al_{201}$ NP-benzene system, with varying NP-molecule distance, fitted to the coupled oscillator model.** The model and fitting scheme are described in Supplementary Note 1.

# Supplementary Tables

Supplementary Table 1: **Prior distributions of parameters in the Bayesian fitting scheme.** Each prior distribution is either gamma or normally distributed with the following parameters.

*Gamma distributed*

$$\left(\frac{x-x_0}{w}\right)^{A-1}\frac{\exp(-\frac{x-x_0}{w})}{w\Gamma(A)}$$

| **Parameter** | $A$ | $x_0$ | $w$ |
|---|---|---|---|
| $g$ (eV) | 3.5 | 0.001 | 0.1 |
| $\gamma_{\mathrm{ex}}$ (eV) | 3.0 | 0.05 | 0.1 |
| $\sigma_{\varepsilon}$ (eV) | 3.0 | 0.5 | 1.5 |

*Normally distributed*

$$\frac{1}{\sqrt{2\pi w^2}}\exp(-\left(\frac{x-x_0}{w}\right)^2)$$

| **Parameter** | $x_0$ | $\sigma$ |
|---|---|---|
| $a$ (1/eV) | 320 | 20 |
| $\omega_{\mathrm{ex}}$ (eV) | 7.0 | 1.0 |
| $\omega_{\mathrm{pl}}$ (eV) | 7.5 | 1.0 |
| $\gamma_{\mathrm{pl}}$ (eV) | 1.1 | 0.4 |

# Supplementary Notes

**Supplementary Note 1: Fitting of spectra.** The spectra of the coupled nanoparticle/molecule systems $\sigma_{\mathrm{abs}}(\omega)$ were fitted using a coupled oscillator model

$$\sigma^{(\mathrm{co})}_{\mathrm{abs}}(\omega) = a\omega\Im\left[\frac{\omega_{\mathrm{ex}}^2 - (\omega + i\gamma_{\mathrm{ex}}/2)^2}{\left(\omega_{\mathrm{ex}}^2 - (\omega + i\gamma_{\mathrm{ex}}/2)^2\right)\left(\omega_{\mathrm{pl}}^2 - (\omega + i\gamma_{\mathrm{pl}}/2)^2\right) - 4g^2\omega^2}\right], \tag{1}$$

where $a$ is an amplitude, $\omega_{\mathrm{ex}}$ and $\gamma_{\mathrm{ex}}$ the exciton resonance frequency and width, $\omega_{\mathrm{pl}}$ and $\gamma_{\mathrm{pl}}$ the plasmon resonance frequency and width and $g$ the coupling strength. These parameters of interest are denoted

$$\boldsymbol{\theta} = (g, a, \omega_{\mathrm{ex}}, \gamma_{\mathrm{ex}}, \omega_{\mathrm{pl}}, \gamma_{\mathrm{pl}}). \tag{2}$$

An additional parameter $\sigma_\varepsilon^2$, which is not of direct interest, is introduced as a fitting error.

We exploited a Bayesian statistics framework, where we calculated the posterior probability distribution $p(\boldsymbol{\theta}, \sigma_\varepsilon^2|\sigma_{\mathrm{abs}}(\omega))$ of parameters $\boldsymbol{\theta}$ given a spectrum $\sigma_{\mathrm{abs}}(\omega)$. The posterior probability is given by Bayes' rule

$$p(\boldsymbol{\theta}, \sigma_\varepsilon^2|\sigma_{\mathrm{abs}}(\omega)) = \frac{p(\sigma_{\mathrm{abs}}(\omega)|\boldsymbol{\theta}, \sigma_\varepsilon^2)p(\boldsymbol{\theta}, \sigma_\varepsilon^2)}{p(\sigma_{\mathrm{abs}}(\omega))}, \tag{3}$$

where $p(\sigma_{\mathrm{abs}}(\omega)|\boldsymbol{\theta}, \sigma_\varepsilon^2)$ is the likelihood of the data, $p(\boldsymbol{\theta}, \sigma_\varepsilon^2)$ the prior probability distribution of the parameters and $p(\sigma_{\mathrm{abs}}(\omega))$ the marginal likelihood which does not need to be explicitly computed due to norm constraints on probability.

To define the likelihood, we postulated that the fitting error $\sigma_{\mathrm{abs}}(\omega) - \sigma^{(\mathrm{co})}_{\mathrm{abs}}(\omega)$ at every point $5.0\,\mathrm{eV} \leq \omega \leq 8.5\,\mathrm{eV}$ is normally distributed with mean zero and variance $\sigma_\varepsilon^2$. Thus the likelihood is

$$p(\sigma_{\mathrm{abs}}(\omega)|\boldsymbol{\theta}, \sigma_\varepsilon^2) = \Pi_{\omega=5\,\mathrm{eV}}^{8.5\,\mathrm{eV}}\left(\frac{1}{2\pi\sigma_\varepsilon^2}\right)\exp\left[-\frac{1}{2}\frac{\left|\sigma_{\mathrm{abs}}(\omega) - \sigma^{(\mathrm{co})}_{\mathrm{abs}}(\omega)\right|^2}{\sigma_\varepsilon^2}\right] \tag{4}$$

The prior distribution of parameters $p(\boldsymbol{\theta}, \sigma_\varepsilon^2)$ was defined as the product of prior distributions of the individual parameters. The prior distributions of the individual parameters are normal or gamma distributions with parameters specified in Supplementary Table 1.

For each fitted spectrum, the posterior distribution was sampled using a Markov chain Monte Carlo ensemble sampler implemented in the emcee package. The ensemble of 100 walkers was run for 15000 steps, with the first 10000 steps discarded as a burn-in phase. Starting positions for the 100 walkers were generated by drawing random samples of the parameters, keeping a few of the random parameters fixed and relaxing the other by performing an ordinary least squares fit.

For each spectrum, the mean of the parameters during the final 5000 Monte Carlo steps were extracted. These values, together with uncertainties as 25th and 75th percentiles, are shown in Supplementary Figure 1. The function (1) is plotted using the extracted parameters together with corresponding spectra in Supplementary Figure 2.
